# Supplementary material for: Simulation-Aided Policy Tuning for Black-Box Robot Learning
Source: arXiv:2411.14246 source file (2024-11-21)
Supplement: Supplementary file 1 [file appendix.tex]

%\section*{Appendix}
%The SE kernel is given as
%\begin{align*}
%K(\theta_1, \theta_2)= \nu^2 \exp \left(-\frac{1}{2}(\theta_1-\theta_2)\tran \lambda (\theta_1-\theta_2) \right),
%\end{align*} 
%where the lengthscale matrix $\lambda \in \mathbb{R}^{d\times d}$ could be any positive-semidefinite matrix, but in practice it is often chosen to be a diagonal one $\lambda = \text{diag}(1/\ell_1^2, \dots, 1/\ell_d^2)$.
%The derivative of the kernel with respect to the first argument is given by
%\begin{align*}
%\frac{\partial K(\theta_1, \theta_2)}{\partial \theta_1} &= -\lambda(\theta_1-\theta_2)K(\theta_1,\theta_2).
%\end{align*}
%The derivative of the SE-kernel with respect to the second argument is given by
%\begin{align*}
%\frac{\partial K(\theta_1, \theta_2)}{\partial \theta_2} &= - \frac{\partial K(\theta_1, \theta_2)}{\partial \theta_1}= \lambda(\theta_1-\theta_2)K(\theta_1,\theta_2).
%\end{align*}
%For the second derivative we obtain
%\begin{align*}
%\frac{\partial^2 K(\theta_1, \theta_2)}{\partial \theta_1 \partial \theta_2} &= \lambda \left(I - (\theta_1 - \theta_2)(\theta_1-\theta_2)\tran \lambda \right)K(\theta_1,\theta_2).
%\end{align*}
